# Supplementary material for: Short Paper: Atomic Execution is Not Enough for Arbitrage Profit Extraction in Shared Sequencers
Source: arXiv:2410.11552 source file (2025-03-02)
Supplement: Supplementary file 1 [file 9-appendix.tex]

\section{Appendix p-1}
